# Supplementary material for: Energy-efficient Deployment of Deep Learning Applications on Cortex-M based Microcontrollers using Deep Compression
Source: arXiv:2205.10369 source file (2023-07-13)
Supplement: Supplementary file 1 [file appendix.tex]

\section{Deployment Results}
\label{app:add_deploy_results}
